# Supplementary material for: Whose Boat Does it Float? Improving Personalization in Preference Tuning via Inferred User Personas
Source: arXiv:2501.11549 source file (2025-06-01)
Supplement: Supplementary file 2 [file persona_prefs.tex]

\begin{figure*}
    \centering
    \includegraphics[width=\linewidth]{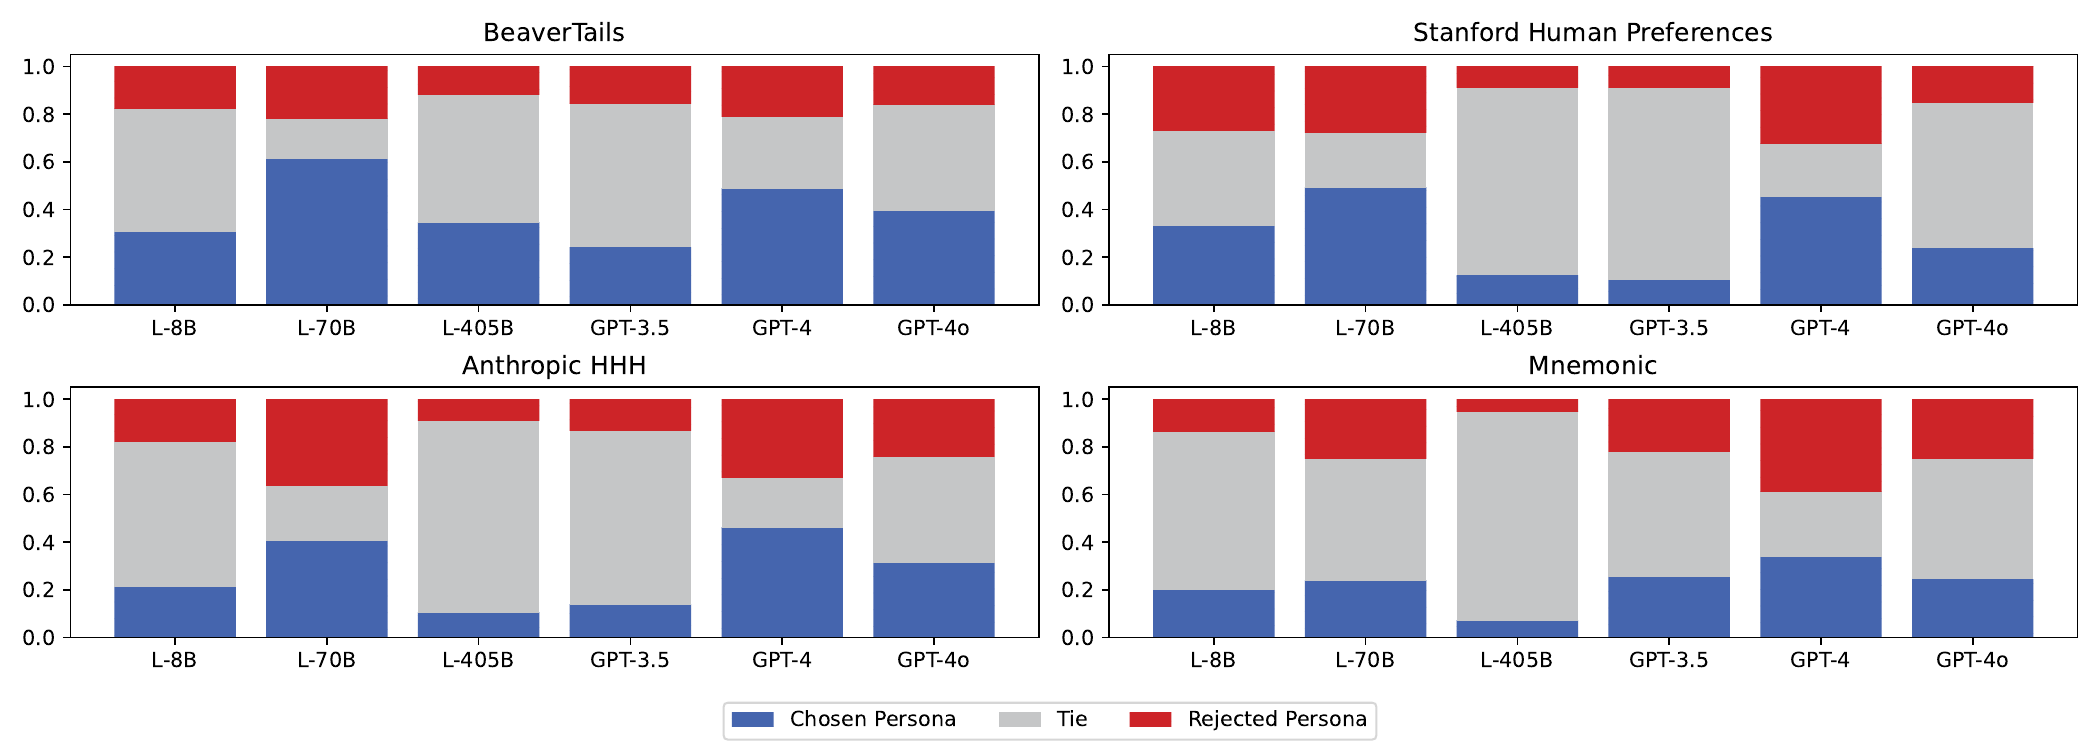}
        \caption{LLM judgments of their own inferred chosen and rejected personas. LLMs often determine that the chosen and rejected personas are of equal quality, reinforcing that rejected responses have valid reasons to be preferred.}
    \label{fig:persona_prefs}
\end{figure*}
