# Supplementary material for: Whose Boat Does it Float? Improving Personalization in Preference Tuning via Inferred User Personas
Source: arXiv:2501.11549 source file (2025-06-01)
Supplement: Supplementary file 3 [file response_type.tex]

\begin{table*}[t]
\small
\centering
\setlength{\tabcolsep}{1.5pt}
\fontsize{7}{8}\selectfont{
\begin{tabular}{@{}ccccccccccc@{}}
\multicolumn{1}{l}{} & \multicolumn{1}{l}{}& \multicolumn{3}{c}{\textit{BeaverTails}}& \multicolumn{3}{c}{\textit{Anthropic HHH}}& \multicolumn{3}{c}{\textit{Mnemonic}} \\ \toprule
$\pi_A$ & \multicolumn{1}{c|}{$\pi_B$} & Person. W/T/L & Quality W/T/L & \multicolumn{1}{c|}{\score} & Person. W/T/L & Quality W/T/L & \multicolumn{1}{c|}{\score} & Person. W/T/L & Quality W/T/L & \multicolumn{1}{c}{\score} \\ \midrule
\multirow{1}{*}{\textsc{DPO}+$\mathcal{P}_{retr, \texttt{C}}$} & \multicolumn{1}{c|}{\textsc{PT}+$\mathcal{P}_{retr, \texttt{C}}$} & \textbf{45.7}/29.9/24.4 & \textbf{41.3}/28.5/30.3 &\multicolumn{1}{c|}{\textcolor{OliveGreen}{+22.8}}& \textbf{42.4}/23.6/34.0 & \textbf{35.2}/30.8/34.0 &\multicolumn{1}{c|}{\textcolor{OliveGreen}{+6.4}}& \textbf{42.0}/28.8/29.2 & \textbf{40.6}/30.4/29.0 &\multicolumn{1}{c}{\textcolor{OliveGreen}{+17.3}}
\\
\multirow{1}{*}{\textsc{DPO}+$\mathcal{P}_{gold, \texttt{C}}$} & \multicolumn{1}{c|}{\textsc{PT}+$\mathcal{P}_{gold, \texttt{C}}$} & \textbf{43.1}/28.3/28.7 & \textbf{38.3}/31.3/30.5 &\multicolumn{1}{c|}{\textcolor{OliveGreen}{+15.7}}& \textbf{41.9}/25.3/32.9 & \textbf{38.7}/26.9/34.5 &\multicolumn{1}{c|}{\textcolor{OliveGreen}{+8.9}}& --- & --- &\multicolumn{1}{c}{---}
\\ \midrule
\multirow{1}{*}{\textsc{DPO}+$\mathcal{P}_{retr, \texttt{R}}$} & \multicolumn{1}{c|}{\textsc{PT}+$\mathcal{P}_{retr, \texttt{R}}$} & \textbf{47.1}/33.5/19.4 & \textbf{38.9}/33.9/27.3 &\multicolumn{1}{c|}{\textcolor{OliveGreen}{+29.6}}& \textbf{54.6}/23.0/22.4 & \textbf{52.4}/23.2/24.4 &\multicolumn{1}{c|}{\textcolor{OliveGreen}{+39.1}}& \textbf{41.4}/26.8/31.8 & \textbf{39.2}/32.2/28.6 &\multicolumn{1}{c}{\textcolor{OliveGreen}{+14.4}}
\\
\multirow{1}{*}{\textsc{DPO}+$\mathcal{P}_{gold, \texttt{R}}$} & \multicolumn{1}{c|}{\textsc{PT}+$\mathcal{P}_{gold, \texttt{R}}$} & \textbf{47.9}/30.7/21.4 & \textbf{35.5}/35.7/28.9 &\multicolumn{1}{c|}{\textcolor{OliveGreen}{+24.2}}& \textbf{47.6}/25.7/26.7 & \textbf{48.2}/25.3/26.5 &\multicolumn{1}{c|}{\textcolor{OliveGreen}{+28.6}}& --- & --- &\multicolumn{1}{c}{---}
\\ \bottomrule
 \end{tabular}
}
 \caption{Comparison of response type on personalization and quality 
}
 \label{table:response_type}
 \end{table*}
